# Supplementary material for: Atomic-detailed milestones along the folding trajectory of protein G
Source: arXiv:0905.2875 source file (2009-05-18)
Supplement: Supplementary file 1 [file supmat.pdf]

**Futher details on the Methods**

**Choice of the driving coordinate.** A critical choice in using the ABMD algorithm is that of the driving coordinate (DC). The more it is correlated with the actual reaction coordinate, the larger one can set the damping constant $\alpha$ without the risk of trapping the trajectory in a dead--end, and the faster the simulation becomes. While $d_{CM}$ proves to be a good representation of the DC, trajectories driven by RMSD or dRMSD did not display any folding event in a set of test simulations. In fact, RMSD and dRMSD (but also the number of H-bonds and the radius of gyration) are correlated with $d_{CM}$ only in the neighbourhood of the native state, but loose this correlation as the system moves towards unfolded conformations (cf. Fig 2 in Supplementary Materials). On the other hand, neither $d_{CM}$ is the actual reaction coordinate, since the folding probability $p_{fold}$ from conformations close to the transition state is not monotonic with respect to this quantity. A more efficient coordinate in this region is the RMSD between the helix and the second hairpin (see upper panel in Fig. 4), as expected from the fact that the lack of contacts between the helix and the second hairpin is a distinctive feature of the transition state (cf. Fig. 3).

**Committors and φ-values.** To validate the generated trajectories and to identify the transition state we have analyzed the distribution of the associated commitment probability (*1*). A series of putative structure were extracted from the trajectory and then simulated twenty times for 10 ns with different starting velocities. The commitment probability $P_i$ is the probability of reaching the native or the denatured basin in short MD trajectories starting from a configuration in which the value of driving coordinate is in the neighborhood of the point i. In particular we calculate $p_{fold}$, that is the probability for the system to reach the native state basins. The native state basin is defined as the region of the conformational space for which the RMSD calculated with respect of the helix and the second hairpin is less than 2.6Å, and with $d_{CM} < 7.5$ .

φ-values for the transition state conformations were calculated as in refs. (*2-4*). In particular, for a configuration at time *t*, we define the calculated φ-value of residue *I* as

$$\phi_I^{calc}(t) = \frac{N_I(t)}{N_I^{nat}},$$

where $N_I$ is the number of native contacts made by the heavy atoms of the side chain of residue *I* and is given by:

$$N_I = \sum_{i \in I}^{M} \sum_{j \notin I}^{M} \psi\left(r_{ij} - r_c\right) \Delta_{ij}(Q)$$

with

$$\psi(r) = \frac{1}{1 + e^{\beta r}}$$

where *M* is the number of heavy atoms in the side chains of the protein, $r_{ij}$ is as usual the distance between atom i and j, $r_c = 0.55\ nm$, $\beta = 50\ nm^{-1}$ and $\Delta_{ij}(Q)$ is equal 1 if atoms i and j are closer than 0.55 nm in the native structure and belongs to residues at least two residues apart in the sequence, and is equal to zero otherwise.

**Homopolymer sequence of events.** To generate the $M_{ij}$ matrix for an homopolymer we define a time constant for each pair of contacts which depends only on the distance of the two amino acids along the chain, that is $\tau_1 = \tau_0(i-j)^{1.5}$ and $\tau_2 = \tau_0(k-l)^{1.5}$, where $\tau_0$ is an immaterial time constant and i, j, k, l are index over the list of residue. The time at which each pair of contacts is formed in a trajectory is a random number extracted from an exponential distribution (i.e. $e^{-t/\tau 1}$ and $e^{-t/\tau 2}$). The realization of the trajectory was repeated 8 times.

**References**


1. Geissler, P. L., Dellago, C., & Chandler, D. (1999) *J. Phys. Chem. B* **103,** 3706-3710.
2. Zhou, R., Berne, B. J., & Germain, R. (2001) *Proc. Natl. Acad. Sci. USA* **98,** 14931-13936.
3. Paci, E., Vendruscolo, M., Dobson, C. M., & Karplus, M. (2002) *J. Mol. Biol.* **324,** 151-163.
4. Calosci, N., Chi, C., Richter, B., Camilloni, C., Engstrom, E., Eklund, L., Travaglini-Allocatelli, C., Gianni, S., Vendruscolo, M., & Jemth, P. (2008) *Proc. Natl. Acad. Sci. USA* **105,** 19240-19245.

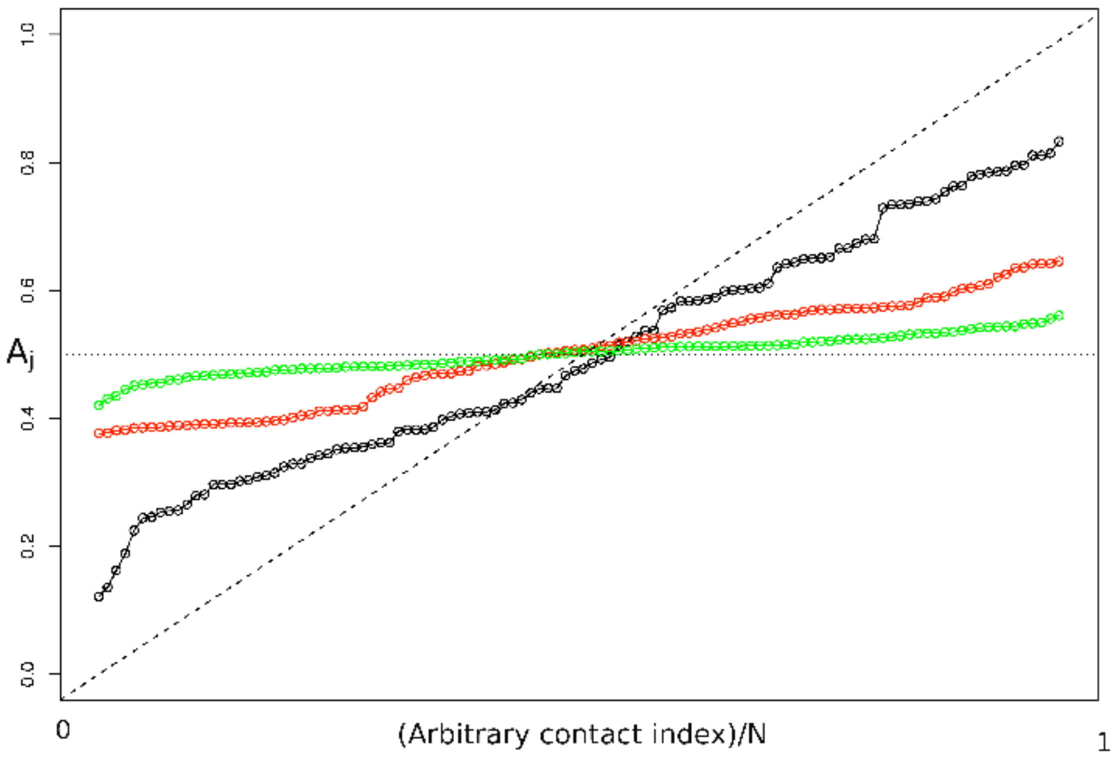


Figure S1: The probability that each contact is formed after all the others, ordered according to their increasing values (black open circles curve). The figure also displays two control curves, one associated with a random matrix, describing a non–hierarchical folding mechanism (green open circles curve) and one associated with the results of an homopolymeric model (red open circles curve). The straight dashed curve illustrates the behavior of the values of $A_j$ associated with a deterministic hierarchical series of folding event, while the horizontal dotted line that associated with a fully cooperative transition.

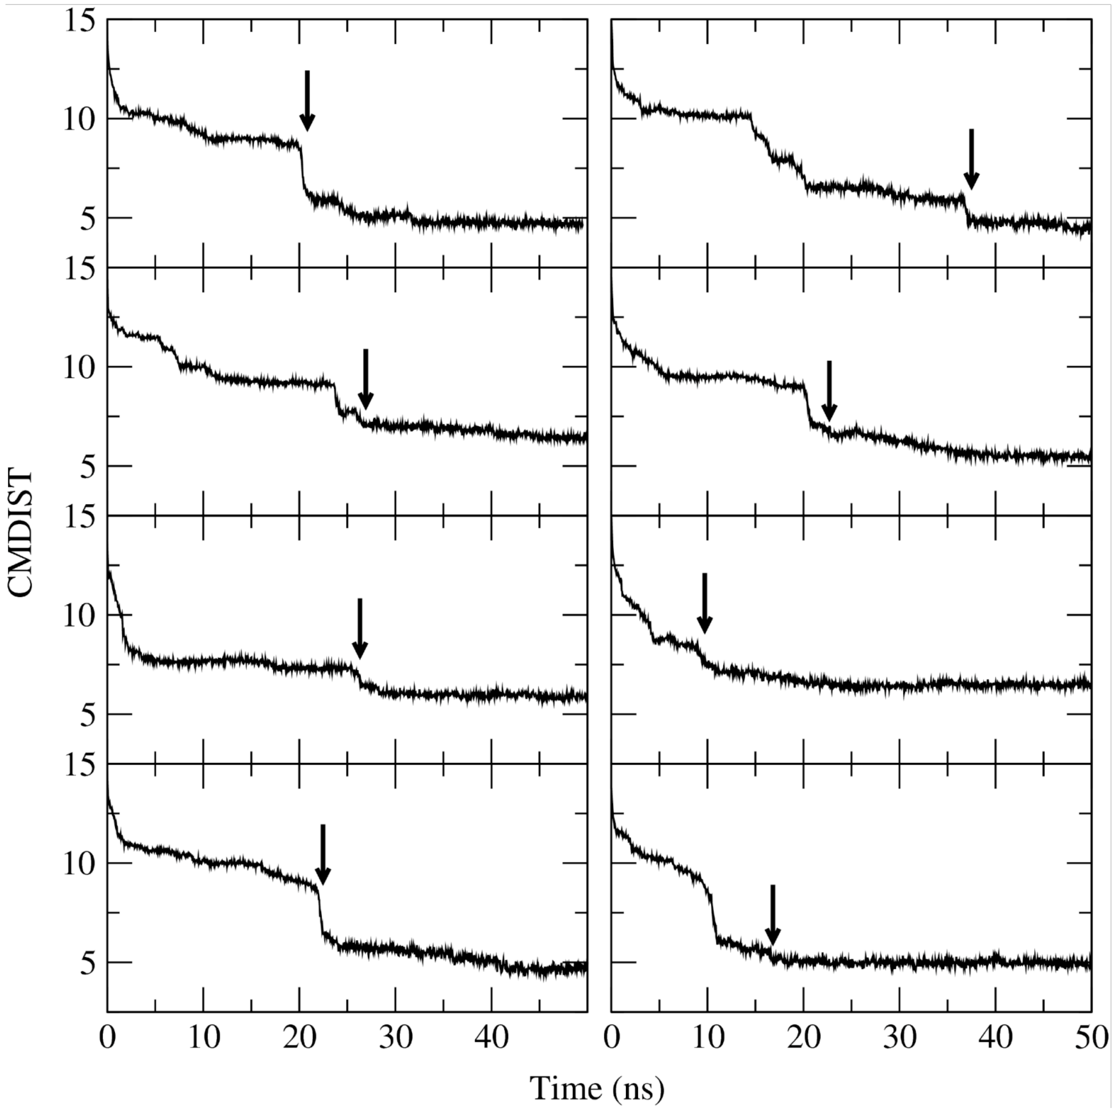


Figure S2: The value of the driving coordinate $d_{CM}$ for the eight folding trajectories. The arrows indicate the transition states.

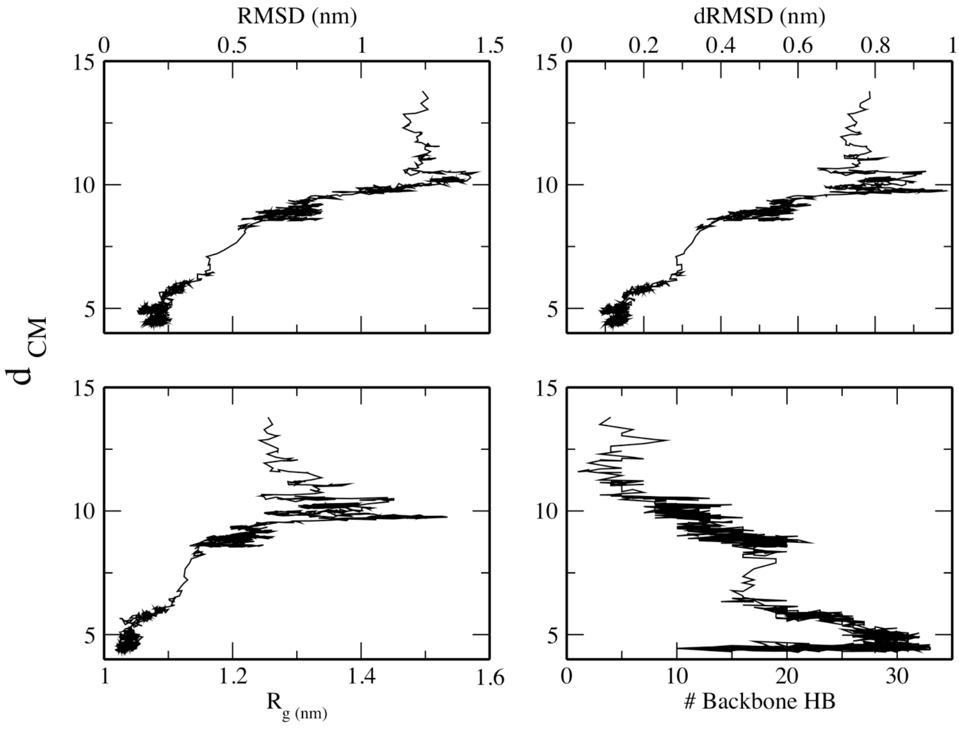


Figure S3: The first folding trajectory (cf. Fig. S2) plotted with respect to different coordinates of the protein ($d_{CM}$, RMSD, dRMSD, radius of gyration $R_g$, number of backbone-backbone hydrogen bonds), to highlight the correlations between them.
